# Supplementary material for: Union and Intersection of all Justifications
Source: arXiv:2109.11216 source file (2021-09-23)
Supplement: Supplementary file 1 [file appendix.tex]

% !TEX root =  dl21.tex

%\clearpage

%\backmatter
\appendix

\section{Detailed Figures}
\begin{figure}[H]
\ffigbox{%
  \includegraphics[width=0.9\textwidth]{fig/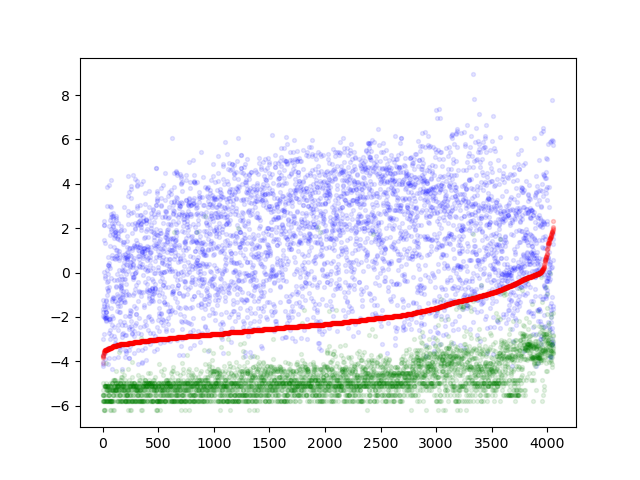} 
}{%
  \caption{Comparison of three methods for computing the union for \ALC-ontologies when there exist several justifications (Same as Fig.~\ref{compare-union-non-trivial})}
}

\ffigbox{%
  \includegraphics[width=0.9\textwidth]{fig/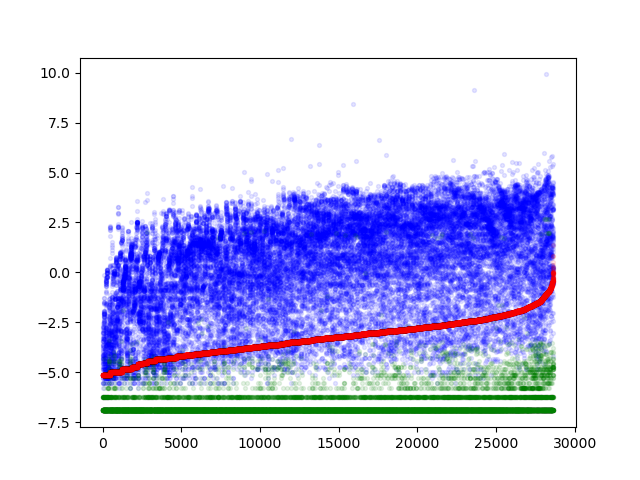} 
}{%
  \caption{Comparison of three methods for computing the union for \ALC-ontologies when there exist only one justification (Same as Fig.~ \ref{compare-union-trivial})}
}

\end{figure}

\begin{figure}

\ffigbox{%
   \includegraphics[width=0.9\textwidth]{fig/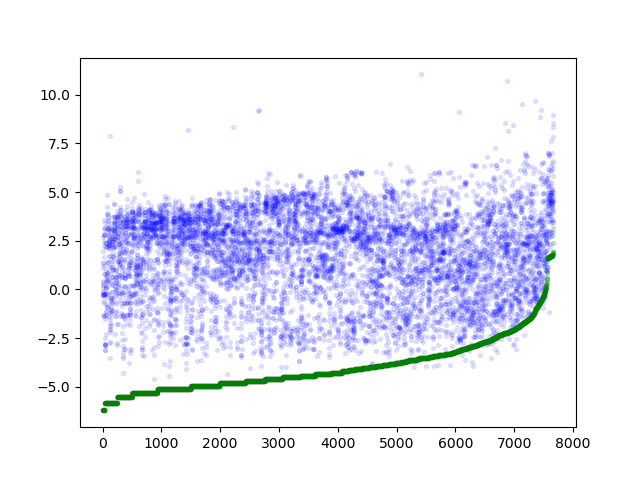}
}{%
 \caption{Comparison of two methods (except MUS-MEM) for computing the union for non \ALC-ontologies when there exist several justifications (Same as Fig.~ \ref{nonALC-non-trivial})}
}
\ffigbox{%
   \includegraphics[width=0.9\textwidth]{fig/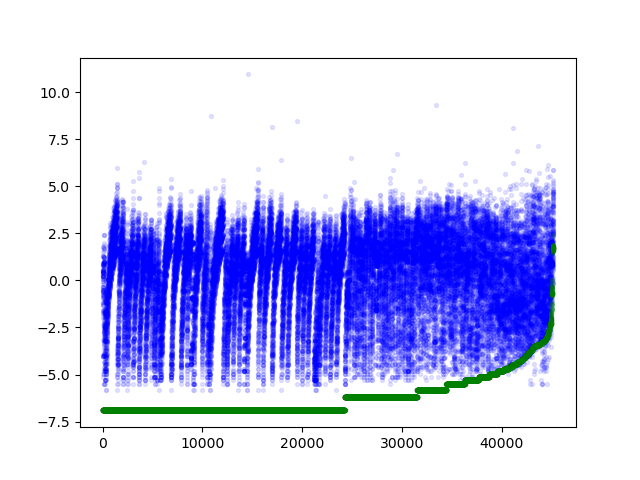} 
}{%
  \caption{Comparison of two methods (except MUS-MEM) for computing the union for non \ALC-ontologies when there exist only one justification (Same as Fig.~ \ref{nonALC-trivial})}
}

\end{figure}

\begin{figure}

\ffigbox{%
   \includegraphics[width=0.9\textwidth]{fig/newcompare_nontrivial_final_nonALC_CJ.png}
}{%
 \caption{relation of ratio $|\Cmc|$/$|\Jmc|$(x-axis) and time cost ratio black-box/OWLAPI( y-axis, without queries with ratio bigger than 1)}
}
\ffigbox{%
   \includegraphics[width=0.9\textwidth]{fig/newcompare_nontrivial_final_nonALC_CU.png} 
}{%
  \caption{relation of ratio $|\Cmc|$/$|\Umc|$(x-axis) and time cost ratio black-box/OWLAPI( y-axis, without queries with ratio bigger than 1)}
}

\end{figure}
\begin{figure}

\ffigbox{%
   \includegraphics[width=0.9\textwidth]{fig/newcompare_nontrivial_final_nonALC_njust.png}
}{%
 \caption{relation of number of justifications(x-axis) and time cost ratio black-box/OWLAPI( y-axis, without queries with ratio bigger than 1)}
}
\end{figure}
